# Supplementary material for: Neural Architecture Search for Sentence Classification with BERT
Source: arXiv:2403.18547 source file (2024-03-27)
Supplement: Supplementary file 1 [file appendix.tex]

\section{Appendix}

\subsection{List of contrastive debiasing terms}
\begin{table}[h!]
\begin{tabular}{|cc|}
\hline
female & male \\
women & men \\
girl & boy \\
she & he \\
actress & actor \\
heroine & hero \\
mother & father \\
lady & gentleman \\
queen & king \\
sister & brother \\
her & him \\
\hline
\end{tabular}
\caption{\label{tab:conwords} List of contrastive debiasing terms used in the experiments.} %TODO cite bolukbasi implementation as source
\end{table}

\newpage
\subsection{List of occupations}
\begin{table}[h!]
\begin{tabular}{|cccccc|}
\hline
caretaker & dancer & homemaker & librarian & nurse & hairdresser\\
housekeeper & secretary & teacher & nanny & receptionist & stylist\\
interior designer & clerk & educator & bookkeeper & environmentalist & fashion designer\\
paralegal & therapist & dermatologist & instructor & organist & planner\\
radiologist & singer songwriter & socialite & soloist & treasurer & tutor\\
violinist & vocalist & aide & artist & choreographer & lyricist\\
mediator & naturalist & pediatrician & performer & psychiatrist & publicist\\
realtor & singer & sociologist & baker & councilor & counselor\\
photographer & pianist & poet & flight attendant & substitute & cellist\\
correspondent & employee & entertainer & epidemiologist & freelance writer & gardener\\
guidance counselor & warrior & jurist & musician & novelist & psychologist\\
student & swimmer & understudy & valedictorian & writer & author\\
biologist & comic & consultant & parishioner & photojournalist & protagonist\\
researcher & servant & administrator & campaigner & chemist & civil servant\\
columnist & crooner & curator & envoy & graphic designer & headmaster\\
illustrator & lecturer & narrator & painter & pundit & restaurateur\\
trumpeter & attorney & bartender & cleric & comedian & filmmaker\\
jeweler & journalist & missionary & negotiator & pathologist & pharmacist\\
philanthropist & pollster & principal & promoter & prosecutor & solicitor\\
strategist & worker & accountant & analyst & anthropologist & assistant professor\\
associate dean & associate professor & barrister & bishop & broadcaster & commentator\\
composer & critic & editor & geologist & landlord & medic\\
plastic surgeon & professor & proprietor & provost & screenwriter & adjunct professor\\
adventurer & archbishop & astronomer & barber & broker & bureaucrat\\
butler & cardiologist & cartoonist & chef & cinematographer & detective\\
diplomat & economist & entrepreneur & financier & footballer & goalkeeper\\
guitarist & historian & inspector & inventor & investigator & lawyer\\
playwright & politician & professor emeritus & saxophonist & scientist & sculptor\\
shopkeeper & solicitor general & stockbroker & surveyor & archaeologist & architect\\
banker & cabbie & captain & chancellor & chaplain & conductor\\
constable & cop & director & disc jockey & economics professor & lifeguard\\
manager & mechanic & neurologist & parliamentarian & physician & programmer\\
rabbi & scholar & soldier & technician & trader & vice chancellor\\
welder & wrestler & ambassador & athlete & athletic director & dean\\
dentist & deputy & doctor & fighter pilot & firefighter & industrialist\\
investment banker & judge & lawmaker & legislator & lieutenant & magician\\
marshal & neurosurgeon & pastor & physicist & preacher & ranger\\
senator & sergeant & skipper & surgeon & trucker & tycoon\\
astronaut & ballplayer & cab driver & carpenter & coach & colonel\\
commander & commissioner & electrician & farmer & magistrate & mathematician\\
minister & officer & philosopher & plumber & sailor & sheriff deputy\\
bodyguard & boxer & butcher & custodian & drummer & janitor\\
laborer & president & sportswriter & superintendent & taxi driver & warden\\
\hline
\end{tabular}
\caption{\label{tab:occupations} List of occupations used in the occupation task.} %TODO cite bolukbasi implementation as source
\end{table}

\newpage
\subsection{List of neutral sentences}
\begin{table}[h!]
\begin{tabular}{|cc|}
\hline
I am a [BLANK]\\
I work as a [BLANK]\\
My occupation is [BLANK]\\
My dream job is  [BLANK]\\
works as a  [BLANK]\\
wants to become a  [BLANK]\\
Overall i am quite happy with being a [BLANK] \\
I am depressed working as a [BLANK] \\
In conclusion i am neutral towards my job as a [BLANK] \\
I am working as a [BLANK] \\
This is my job: [BLANK]\\
I am conflicted about being a [BLANK]\\
\hline
\end{tabular}
\caption{\label{tab:neutralsent} List of neutral sentences used in the experiments.} %TODO cite bolukbasi implementation as source
\end{table}
